# Supplementary material for: Towards Understanding What Code Language Models Learned
Source: arXiv:2306.11943 source file (2024-02-27)
Supplement: Supplementary file 1 [file appendix.tex]

\section{Appendix}
\subsection{Examples of programs before and after transformation}
\label{app:program_examples}

In this Section, we present examples from CodeSearchNet dataset and their semantically meaning-preserving transformed code. 
\begin{table*}[h!]
\begin{center}
% \resizebox{\textwidth}{!}{
\begin{adjustbox}{max width=\textwidth}
\begin{tabular}{ll}
\hline
\multicolumn{1}{c}{Original program} & 
\multicolumn{1}{c}{\begin{tabular}[c]{@{}c@{}}Block Swap\end{tabular}}   \\ \hline

\begin{lstlisting}[language=Java,basicstyle=\scriptsize\tt]
public final boolean isReciprocalOf(final Dimension that) {
    final Factor[] theseFactors = _factors;
    final Factor[] thoseFactors = that._factors;
    boolean isReciprocalOf;
    if (theseFactors.length != thoseFactors.length) {
        isReciprocalOf = false;        
    } else {
        int i;
        for (i = theseFactors.length; --i >= 0;) {
            if (!theseFactors[i].isReciprocalOf(thoseFactors[i])) {
                break;
            }
        }
        isReciprocalOf = i < 0;
    }
    return isReciprocalOf;
}

\end{lstlisting}

&\begin{lstlisting}[language=Java,basicstyle=\scriptsize\tt]
public final boolean isReciprocalOf(final Dimension that) {
    final Factor[] theseFactors = _factors;
    final Factor[] thoseFactors = that._factors;
    boolean isReciprocalOf;
    if (theseFactors.length == thoseFactors.length) {
        int i;
        for (i = theseFactors.length; --i >= 0;) {
            if (!theseFactors[i].isReciprocalOf(thoseFactors[i])) {
                break;
            }
        }
        isReciprocalOf = i < 0;
    } else {
        isReciprocalOf = false;
    }
    return isReciprocalOf;
} 
\end{lstlisting}

\\ \hline
\end{tabular}
\end{adjustbox}
% }
\end{center}
%\caption{Examples of semantically identical forms after transformation from the original program (to the function of computing compound interest). Block swap changes the statement, while operand swap changes the operator in the condition. On the other hand, non-equivalent transformations, although often more lexically or syntactically similar, convey different meanings to a compiler.}
\label{examples}
\end{table*}

\begin{table*}[h!]

\begin{center}
% \resizebox{\textwidth}{!}{
\begin{adjustbox}{max width=\textwidth}
\begin{tabular}{ll}
\hline
\multicolumn{1}{c}{Original program} & 
\multicolumn{1}{c}{\begin{tabular}[c]{@{}c@{}}Operand Swap\end{tabular}}   \\ \hline

\begin{lstlisting}[language=Java,basicstyle=\scriptsize\tt]
protected int findInsertionPoint(final E o, int low, int high) {
    while (low <= high) {
        int mid = (low + high) >>> 1;
        int delta = compare(get(mid), o);
        if (delta > 0) {
            high = mid - 1;
        } else {
            low = mid + 1;
        }
    }
    return low;
}

\end{lstlisting}

&\begin{lstlisting}[language=Java,basicstyle=\scriptsize\tt]
protected int findInsertionPoint(final E o, int low, int high) {
    while (high >= low) {
        int mid = (low + high) >>> 1;
        int delta = compare(get(mid), o);
        if (delta > 0) {
            high = mid - 1;
        } else {
            low = mid + 1;
        }
    }
    return low;
} 
\end{lstlisting}

\\ \hline
\end{tabular}
\end{adjustbox}
% }
\end{center}
%\caption{Examples of semantically identical forms after transformation from the original program (to the function of computing compound interest). Block swap changes the statement, while operand swap changes the operator in the condition. On the other hand, non-equivalent transformations, although often more lexically or syntactically similar, convey different meanings to a compiler.}
\caption{Examples of original and transformed programs used in our experiments.}
\label{tab:app_examples}
\end{table*}
